# Supplementary material for: ThinkRL-Edit: Thinking in Reinforcement Learning for Reasoning-Centric Image Editing
Source: arXiv:2601.03467 source file (2026-02-26)
Supplement: Supplementary file 1 [file X_suppl.tex]

\clearpage
\setcounter{page}{1}
\maketitlesupplementary

% \section{Normal Benchmark}

% \section{T2I}
\begin{figure*}[t]
    \centering
    \includegraphics[width=\linewidth]{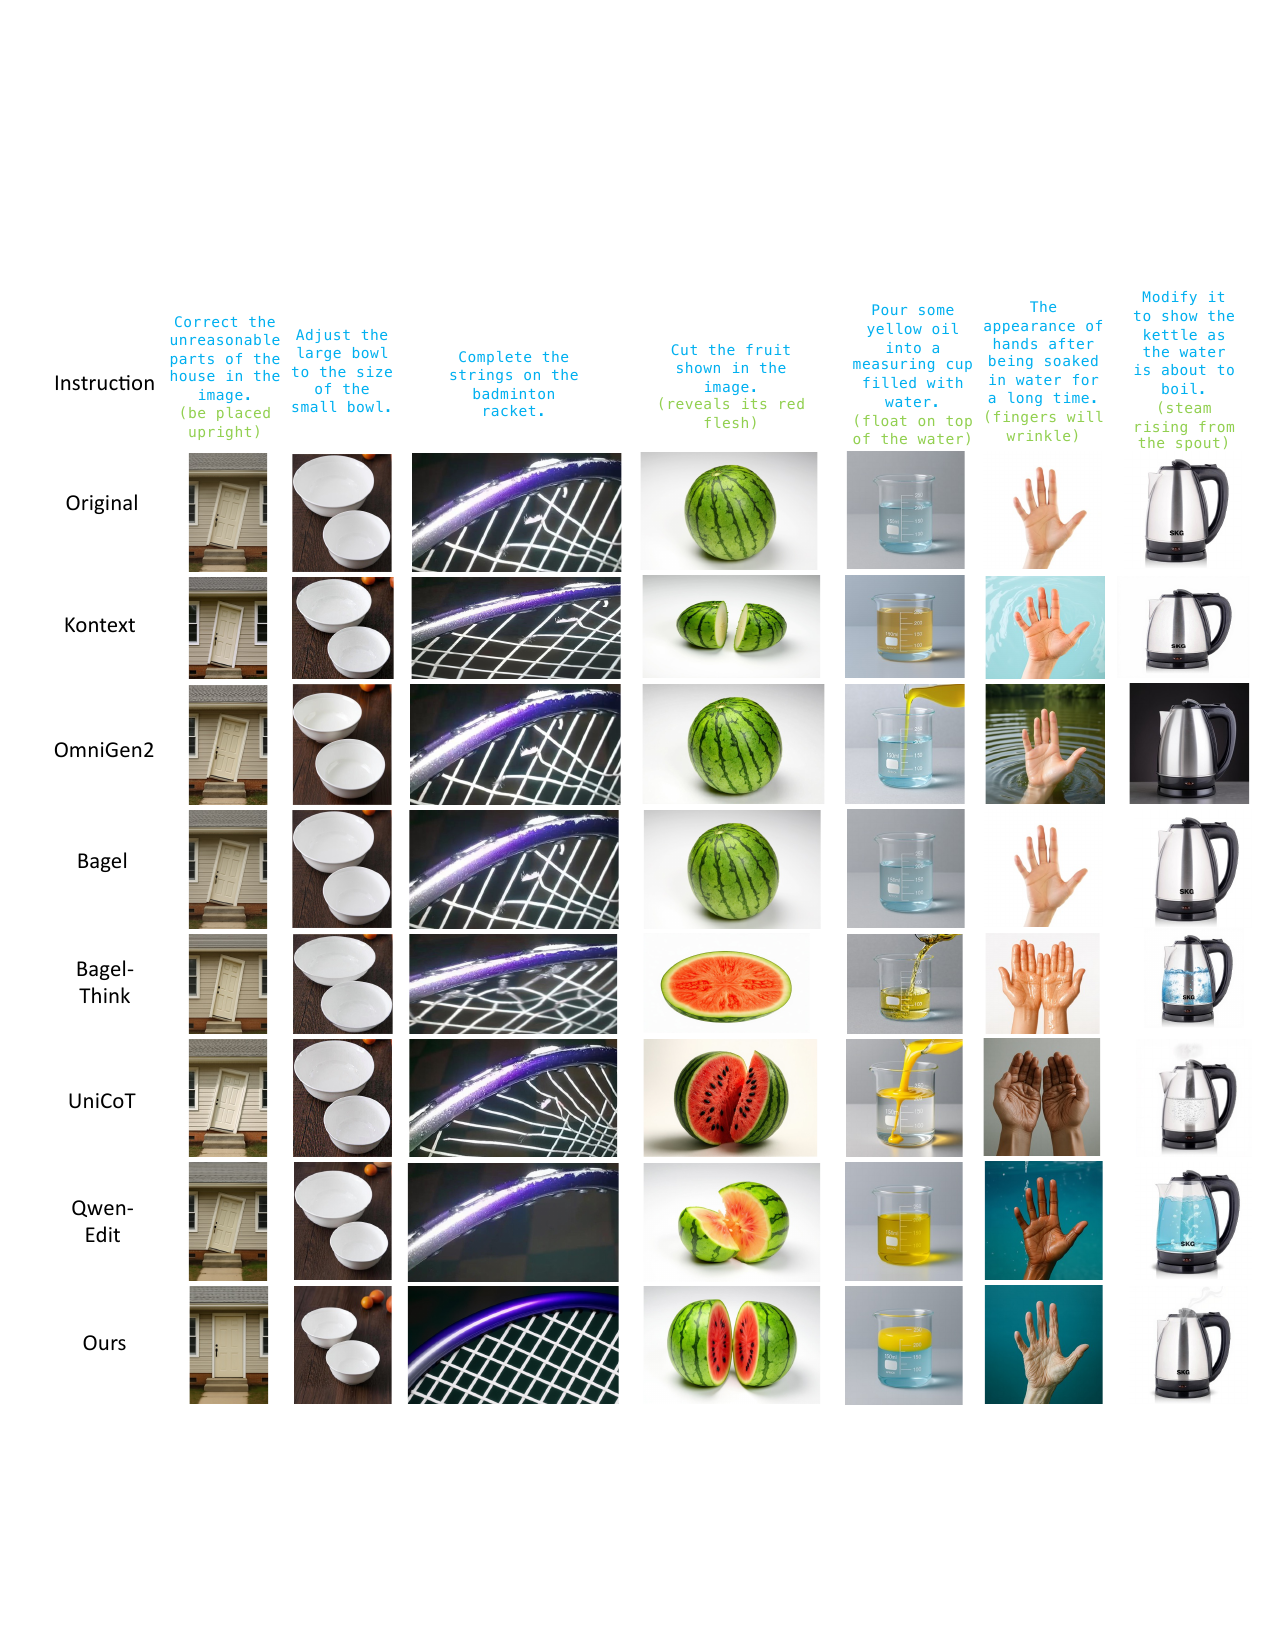}
    % \vspace{-0.3cm}
            \caption{\textbf{More comparison with previous methods.}
    }
    % \vspace{-0.6cm}
    \label{fig:add}
\end{figure*}
\section{Experiment Details}
We train all modules of Qwen-Edit with the AdamW optimizer (beta1 = 0.9, beta2 = 0.999, epsilon = 1e-8), using a learning rate of 3e-4, weight decay of 1e-4, group size of 128, and a batch size of 4. For both training-time sampling and inference, we adopt a single-pass schedule consisting of one editing step followed by one reflection-guided editing step, i.e., exactly one edit and one reflection-then-refine per sample.

\section{More Comparison}
As shown in \cref{fig:add}, we present additional comparisons with previous methods. Compared to the baselines, our approach preserves strong fidelity to reasoning-centric context while enabling precise visual edits. It achieves high instruction adherence, substantial image consistency, and plausible visual transitions.

\section{Details of User Study}
To further assess the effectiveness of our approach, we conduct a controlled human evaluation against representative image editing baselines. We recruit 20 participants and present them with 24 sets of generated results. Each set includes a reference image and an instruction prompt, alongside edited outputs from different methods produced using the same random seed to ensure comparability.
We evaluate edited images along three dimensions: Instruction Following (IF), Visual Consistency (VC), Visual Quality (VQ).
For each set, participants are asked to select the single best result across all criteria. We then aggregate selections across all sets and participants to compute per-method preference ratios for each dimension. As summarized in \cref{tab:user}, our method achieves substantially higher user preference across all metrics, highlighting its superior instruction adherence, consistency with the source image, and overall visual fidelity.

\section{System Prompt}
In the CoT-based sampling stage, we employ two strategies, planning and reflection. We present the detailed system prompts for both in \cref{plan} and \cref{reflect}: the planning prompt guides decomposition of the reference image and instruction into concrete, executable editing steps, whereas the reflection prompt evaluates the initial edit for instruction adherence, visual consistency, and visual quality, identifies errors or artifacts, and proposes minimal, effective corrections to produce a refined second-pass edit directive.

\begin{table*}[htbp]
  \centering
  \caption{\textbf{System Prompt for Planning}}
  
  \begin{tabular}{c}
    \toprule
 \begin{lstlisting}
system_prompt_planning = """
You are a Visual Instruction Rewriter for multimodal image editing models.
Your task is to rewrite a user's image editing instruction so that an image editing model can easily understand and correctly perform the edit. 

You will be given:
1. **Input Image**: the original image before editing <image>
2. **Instruction**: the original user instruction describing the desired edit

### Your Objective
- Clarify and Ground the Instruction: Make all edits visually explicit, using concrete visual concepts (objects, positions, colors, lighting, textures, shapes, materials).
- Add a Factual Rationale (if needed): If the instruction requires external or domain knowledge (e.g., physical realism, color consistency, biological accuracy, material reflection, geometry), provide a short explanation under the section 'Factual Rationale', describing what the correct result should visually look like

### Output Format
Provide the rewrited instruction in the following JSON format:
{{
"Rewrited": "" 
}}

### Example
Instruction: This bread after being left for a long time
{{
"Rewrited": "Make the bread appear moldy. It should be covered in splotches of green, black, and white fuzzy mold, particularly on the crusts and cut surfaces, indicating significant spoilage from being left out for a long time."
}}

"""
\end{lstlisting}
\\
    \bottomrule
  \end{tabular}
    \label{plan}
\end{table*}

\begin{table*}[htbp]
  \centering
  \caption{\textbf{System Prompt for Reflection}}
  
  \begin{tabular}{c}
    \toprule
 \begin{lstlisting}
system_prompt_reflection = """
You are a professional AI image specialist. Your role is to critically determine an AI-generated edited image by comparing it to the original image and a given editing instruction. You must identify exactly what parts of the instruction were fulfilled, partially fulfilled, or missing, and provide concrete suggestions for the next edit to fully satisfy the instruction.

You will be given:
1. **Image A**: the original image <image>.
2. **Image B**: the edited image <image>.
3. **Editing Instruction**: a directive describing the intended modification to Image A to produce Image B. {instruction} 

### Your Objectives
- Detect all visible differences between Image A and Image B accurately.
- Determine whether these differences match the editing instruction exactly.
- Identify missing, incorrect, or insufficient edits.
- Provide clear, actionable suggestions for the next editing attempt to fully fulfill the instruction.
- Ignore unrelated visual changes; focus strictly on the instruction.
- Do not provide any scores.

### Reasoning Steps
- Detect Difference: Describe all visible changes between Image A and Image B (size, shape, color, position, texture, presence/absence of objects, etc.), without referencing the instruction yet.
- Instruction Match: Compare actual changes to expected changes:
   - Was the correct object modified (not replaced)?
   - Was the requested attribute (color, size, position, texture, etc.) modified correctly?
   - Was the degree/extent of modification accurate?
- Edit Suggestion: Provide specific instructions for the next edit to fix missing or incorrect modifications. Be concrete and concise; target only the unsatisfied parts of the instruction.

### Output Format
Return your results in strict JSON:
{{
"edit_suggestion": ""
}}

### Example
Instruction: Adjust the size of the apple to match the size of the watermelon
{{
"edit_suggestion": "Increase the apple's size further so that its height and overall volume visually match the watermelon."
}}
"""
\end{lstlisting}
\\
    \bottomrule
  \end{tabular}
    \label{reflect}
\end{table*}

\section{Ethics Statement}
Our primary objective in this work is to empower novice users to generate visual content in a creative and flexible manner. However, we recognize the potential risks associated with the misuse of this technology in generating fake or harmful content. As such, we emphasize the importance of developing and implementing robust tools to detect biases and identify malicious use cases, ensuring the safe and equitable deployment of this technology.

\section{Reproducibility Statement}
To ensure the reproducibility of our method, we make the following efforts: (1) The training and inference code, along with the trained model weights, will be made publicly available. (2) Detailed training procedures are provided in the appendix, designed for ease of use. (3) We also include comprehensive information on the human evaluation setups.

\section{LLM Usage Statement}
Large Language Models (LLMs), specifically OpenAI's GPT-5, were utilized as a general-purpose assistive tool during the preparation of this paper. The model was primarily employed for:
(1) Language polishing – refining grammar, enhancing clarity, and adjusting tone to meet academic writing standards.
(2) Formatting support – generating LaTeX table templates, figure captions, and ensuring consistent section structuring.

All core research activities—encompassing problem formulation, theoretical development, model design, experimentation, analysis, and conclusions—were conceived and executed entirely by the authors. The LLM was not involved in generating original research ideas, deriving results, or writing substantive scientific content.
