# Supplementary material for: ThinkRL-Edit: Thinking in Reinforcement Learning for Reasoning-Centric Image Editing
Source: arXiv:2601.03467 source file (2026-02-26)
Supplement: Supplementary file 2 [file appendix.tex]

\section{Hello World}
%\subsection{Hello World}
